# Supplementary material for: Dhara: Evidence-Oriented Retrieval for Indian Knowledge Systems
Source: arXiv:2611.11197 source file (2026-11-08)
Supplement: Supplementary file 1 [file supplementary-labels.tex]

\makeatletter
\newlabel{supp-app:representation-results}{{S1}{1}{Additional Experiment 1 Results}{section.1}{}}
\newlabel{supp-fig:compactencoder}{{S1}{2}{Supplementary neural-model comparison, including the compact all-MiniLM-L6-v2 encoder. Double slashes mark truncated axes}{figure.caption.1}{}}
\newlabel{supp-fig:depth-precision}{{S2}{3}{Experiment 1 category mean Precision across retrieval cutoffs $k=20,50,100,500,1000$. Double slashes mark truncated axes}{figure.caption.2}{}}
\newlabel{supp-fig:depth-recall}{{S3}{4}{Experiment 1 category mean Recall across retrieval cutoffs $k=20,50,100,500,1000$. Double slashes mark truncated axes}{figure.caption.3}{}}
\newlabel{supp-fig:depth-f1}{{S4}{5}{Experiment 1 category mean F1 across retrieval cutoffs $k=20,50,100,500,1000$. Double slashes mark truncated axes}{figure.caption.4}{}}
\newlabel{supp-fig:depth-ndcg}{{S5}{6}{Experiment 1 category mean nDCG across retrieval cutoffs $k=20,50,100,500,1000$. Double slashes mark truncated axes}{figure.caption.5}{}}
\newlabel{supp-fig:depth-mrr}{{S6}{7}{Experiment 1 category mean MRR across retrieval cutoffs $k=20,50,100,500,1000$. Double slashes mark truncated axes}{figure.caption.6}{}}
\newlabel{supp-fig:depth-complete}{{S7}{8}{Experiment 1 complete-evidence scores across retrieval cutoffs for T06 ($n=19$) and T07 ($n=15$). Double slashes mark truncated axes}{figure.caption.7}{}}
\newlabel{supp-fig:representationtiming}{{S8}{8}{Experiment 1 category mean direct retrieval time, using the same GPU and timing scope for all three models}{figure.caption.8}{}}
\newlabel{supp-app:sv-results}{{S2}{9}{Additional Component Results}{section.2}{}}
\newlabel{supp-fig:geminioff}{{S9}{10}{EN+SV versus Gemini with FVR disabled. Score pairs show Gemini to EN+SV; bars show changes in percentage points (pp)}{figure.caption.9}{}}
\newlabel{supp-fig:svfvronofffull}{{S10}{11}{FVR effects by category. Score pairs show FVR off to FVR on; bars show changes in percentage points (pp). Each pair shares the ranking before FVR}{figure.caption.10}{}}
\newlabel{supp-tab:novscores1}{{S1}{12}{Component scores for T01-T04}{table.caption.11}{}}
\newlabel{supp-tab:novscores2}{{S2}{13}{Component scores for T05-T08}{table.caption.12}{}}
\newlabel{supp-tab:novscores3}{{S3}{14}{Component scores for T09-T12}{table.caption.13}{}}
\newlabel{supp-tab:novf1}{{S4}{14}{Category-wise F1@10. SV denotes SV matched; B/Q denotes BGE/Qwen; the FVR columns include EN+SV}{table.caption.14}{}}
\newlabel{supp-app:prompts}{{S3}{15}{Natural-Language Prompts}{section.3}{}}
\newlabel{supp-app:entity-extraction}{{S3.1}{15}{Chapter-level entity extraction prompt}{subsection.3.1}{}}
\newlabel{supp-app:ces-generation}{{S3.2}{15}{Chapter-level Entity Notes generation prompt}{subsection.3.2}{}}
\newlabel{supp-app:bes-consolidation}{{S3.3}{16}{Book-level Entity Notes consolidation prompt}{subsection.3.3}{}}
\newlabel{supp-app:verse-extraction}{{S3.4}{16}{Verse-fragment extraction prompt}{subsection.3.4}{}}
\newlabel{supp-app:qwen-reranking}{{S3.5}{17}{Qwen passage-relevance scoring prompt}{subsection.3.5}{}}
\newlabel{supp-app:gemini-prompt}{{S3.6}{17}{Gemini retrieval prompt and permitted sources}{subsection.3.6}{}}
\newlabel{supp-tab:geminisources}{{S5}{18}{The 20 prose-source entries in the Gemini generation prompt}{table.caption.15}{}}
\newlabel{supp-app:gemma-prompts}{{S3.7}{18}{Gemma prompts for source and chunk selection}{subsection.3.7}{}}
\newlabel{supp-app:settings}{{S4}{19}{Implementation and Evaluation Settings}{section.4}{}}
\newlabel{supp-app:retrieval-settings}{{S4.1}{19}{SV component-pipeline settings}{subsection.4.1}{}}
\newlabel{supp-app:bm25-settings}{{S4.2}{19}{BM25 indexing and query settings}{subsection.4.2}{}}
\newlabel{supp-tab:auditsettings}{{S6}{20}{Experiment 2 settings. Both retrieval branches provide $S_q$ source chunks; CombMAX combines their rankings before truncation to the top $S_q$}{table.caption.16}{}}
\newlabel{supp-tab:rerankserving}{{S7}{20}{vLLM reranker serving settings}{table.caption.17}{}}
\newlabel{supp-tab:exp2systems}{{S8}{20}{Experiment 2 systems and their pipeline roles}{table.caption.18}{}}
\newlabel{supp-app:generation-settings}{{S4.3}{21}{Model settings for Entity Notes and fragment extraction}{subsection.4.3}{}}
\newlabel{supp-tab:generationsettings}{{S9}{21}{Entity extraction, Entity Note generation, and FVR activation settings}{table.caption.19}{}}
\newlabel{supp-app:verse-implementation}{{S4.4}{21}{FVR normalization and verse-to-chunk matching}{subsection.4.4}{}}
\newlabel{supp-app:evaluation-fields}{{S4.5}{22}{Question alignment and timing scope}{subsection.4.5}{}}
\newlabel{supp-app:direct-settings}{{S4.6}{22}{Experiment 1 retrieval and hardware settings}{subsection.4.6}{}}
\newlabel{supp-tab:exp1system}{{S10}{22}{Experiment 1 host and software configuration}{table.caption.20}{}}
\newlabel{supp-tocindent-1}{0pt}
\newlabel{supp-tocindent0}{0pt}
\newlabel{supp-tocindent1}{8.54999pt}
\newlabel{supp-tocindent2}{14.71498pt}
\newlabel{supp-tocindent3}{0pt}
\newlabel{supp-app:minilm-settings}{{S4.7}{23}{all-MiniLM-L6-v2 encoder and retrieval settings}{subsection.4.7}{}}
\newlabel{supp-app:gemini-settings}{{S4.8}{23}{Gemini generation and cache settings}{subsection.4.8}{}}
\newlabel{supp-tab:geminisettings}{{S11}{23}{Recorded Gemini generation and cache settings}{table.caption.21}{}}
\newlabel{supp-app:gemini-mapping}{{S4.9}{23}{Gemini source mapping and manual review settings}{subsection.4.9}{}}
\newlabel{supp-tab:gemmamapping}{{S12}{24}{Automatic Gemma mapping settings for location and source-chunk selection}{table.caption.22}{}}
\newlabel{supp-TotPages}{{24}{24}{}{page.24}{}}
\makeatother
